# Supplementary material for: Extended Analysis of "How Child Welfare Workers Reduce Racial Disparities in Algorithmic Decisions"
Source: arXiv:2204.13872 source file (2022-04-29)
Supplement: Supplementary file 1 [file appendixtables.tex]

\begin{table*}[h]
\begin{tabular}{|p{0.5\linewidth} | p{0.5\linewidth}|}
\hline
\cellcolor{tempblue}\textbf{Analysis 1} & \cellcolor{tempviolet}\textbf{Analysis 2} \\ \hline
 Fully automated AFST-only decisions would have screened in 71.0\% of Black children and 51.0\% of white children in discretionary referrals from 2016-18, a racial disparity of 20\%. Over the same time period, workers using the AFST screened in 61.8\% of Black children and 52.8\% of white children, a disparity of 9\%. Thus, worker-AFST decisions reduced disparities in the AFST by 11\%.
& AFST-only decisions would have screened in 67.9\% of Black children and 50.0\% of white children in discretionary referrals from 2016-18, a racial disparity of 17.9\%. Over the same time period, workers using the AFST screened in 50.2\% of Black children and 43.1\% of white children, a disparity of 7.1\%. Thus, worker-AFST decisions reduced disparities in the AFST by 10.8\%. \\ \hline
AFST-only decisions would have had a 13.5\% Black-white disparity in terms of accuracy, compared to 5.4\% for worker-AFST decisions. Thus, worker-AFST were less disparate than the AFST on its own in terms of accuracy. & AFST-only decisions would have had a 13.6\% Black-white disparity in terms of accuracy, compared to 5.8\% for worker-AFST decisions. Thus, worker-AFST were less disparate than the AFST on its own in terms of accuracy. \\ \hline
AFST-only decisions would have been accurate for 51.0\% of all children, versus 46.5\% for worker-AFST decisions. Thus, the AFST on its own would have been more accurate than workers.    &   AFST-only decisions would have been accurate for 48.4\% of all children, versus 50.4\% for worker-AFST decisions. Thus, the AFST on its own would have been slightly less accurate than workers. \\
\hline
\end{tabular}
\caption{Comparison of quantitative findings between Analyses 1 and 2}
\label{tab:findings_comparison}
\end{table*}

\begin{table*}[h]
\begin{tabular}{|p{0.2\linewidth} |p{0.4\linewidth} | p{0.4\linewidth}|}
\hline
& \cellcolor{tempblue}\textbf{Analysis 1} & \cellcolor{tempviolet}\textbf{Analysis 2} \\ \hline
Population data
& PAN\_Retro\_Run\_Referrals\_for\_2014-2016\_provided\_2018-08-29.csv, PAN\_Retro\_Run\_08012016\_07132018.csv\footnotemark
& LIM\_REFERRAL\_CLIENTS\_UNIQapp\_04212022\_v3.csv \\ \hline
Exclusions
& LIM\_REFERRAL\_CLIENTS\_08262021.csv
& LIM\_REFERRAL\_CLIENTS\_UNIQapp\_04212022\_v3.csv \\ \hline
Placements
& PLACEMENTS\_DEID\_FULL\_07232020.csv
& LIM\_PLACEMENTS\_08262021.csv \\ \hline
AFST scores
& PAN\_Retro\_Run\_Referrals\_for\_2014-2016\_provided\_2018-08-29.csv, PAN\_Retro\_Run\_08012016\_07132018.csv, RR\_scorecutoffs.csv, PL\_scorecutoffs.csv
& RETRO\_FILES\_COMBINED\_04212022\_v3.csv\\
\hline
\end{tabular}
\caption{Comparison of data used between Analyses 1 and 2}
\label{tab:data_comparison}
\end{table*}
\footnote{We have not yet confirmed whether these PAN\_Retro files are the same that \citet{goldhaber2019impact} used in their work.}

\begin{table*}[h]
\begin{tabular}{|p{0.5\linewidth} | p{0.5\linewidth}|}
\hline
\cellcolor{tempblue}\textbf{Analysis 1} & \cellcolor{tempviolet}\textbf{Analysis 2} \\ \hline
 \begin{enumerate}
     \item Non-GPS referrals (where REFER\_TYPE\_GPS\_NULL!=1 in PAN\_Retro\_Run\_Referrals\_for\_2014-2016)
    \item Referrals connected to completed cases (CALL\_SCRN\_OUTCOME='Screen Out: **Assessment Completed on Active Family**' in LIM\_REFERRAL\_CLIENTS)
    \item Referrals connected to active cases (CALL\_SCRN\_OUTCOME='Accept: Actively working with this family' in LIM\_REFERRAL\_CLIENTS)
 \end{enumerate} & 
 \begin{enumerate}
     \item Non-GPS referrals (where REF\_TYPE !=  'GPS' in LIM\_REFERRAL\_CLIENTS\_UNIQapp\_04212022\_v3)
    \item Active referrals (where ACTIVE\_FAMILY\_IND=1)
    \item Referrals from truancy court (where TRUANCY\_ONLY\_COURTS\_REF = 1)
    \item Non-children (where ALL\_CHILD != 1)
    \item Intake didn't screen (CALL\_SCRN\_CODE = -9)
    \end{enumerate}\\
\hline
\end{tabular}
\caption{Comparison of data exclusions steps between Analyses 1 and 2}
\label{tab:exclusions_comparison}
\end{table*}

\begin{table*}[h]
\begin{tabular}{|p{0.5\linewidth} | p{0.5\linewidth}|}
\hline
\cellcolor{tempblue}\textbf{Analysis 1} & \cellcolor{tempviolet}\textbf{Analysis 2} \\ \hline
 \begin{enumerate}
     \item white: 'RACE\_WHITE\_NULL']==1 and 'RACE\_BLACK\_NULL', 'RACE\_HISPANIC\_NULL', 'RACE\_NATIVE\_NULL', 'RACE\_ASIAN\_NULL', 'RACE\_OTHER\_NULL', 'RACE\_UNKNOWN\_NULL' = 0 in PAN\_Retro
     \item Black: 'RACE\_BLACK\_NULL'=1 in PAN\_Retro
 \end{enumerate} & 
 \begin{enumerate}
     \item white: RACE == 'White' in LIM\_REFERRAL\_CLIENTS\_UNIQapp\_04212022\_v3
    \item Black: RACE contains 'Black or African American' in LIM\_REFERRAL\_CLIENTS\_UNIQapp\_04212022\_v3
    \end{enumerate}\\
\hline
\end{tabular}
\caption{Comparison of race (Black and white) coding between Analyses 1 and 2}
\label{tab:racecoding_comparison}
\end{table*}
